# Supplementary material for: Privacy Perceptions and Behaviors of Google Personal Account Holders in Saudi Arabia
Source: arXiv:2308.10148 source file (2024-08-07)
Supplement: Supplementary file 1 [file questions_demo.tex]

\subsection{Demographic Questions}
\begin{itemize}
    \item \textbf{Q. 1} What is your nationality?  \par
    \textbf{Answers:} \begin{inparaitem}[$\circ$]\item \quotes{Saudi,} \item \quotes{Other (*required: please specify)} \end{inparaitem} \par 
    \vspace{4pt}

    \item \textbf{Q. 2} What is your gender? \par 
    \textbf{Answers:} \begin{inparaitem}[$\circ$]\item \quotes{Female,} \item \quotes{Male} \end{inparaitem} \par  
    \vspace{4pt}

    \item \textbf{Q. 3} What is your marital status? \par 
    \textbf{Answers:} \begin{inparaitem}[$\circ$]\item \quotes{Single,} \item \quotes{Married,} \item \quotes{Divorced,} \item \quotes{Widow,} \item \quotes{I prefer not to answer,} \item \quotes{Other (*required: please specify)} \end{inparaitem} \par  
    \vspace{4pt}

    \item \textbf{Q. 4} Do you have kids? \par 
    \textbf{Answers:} \begin{inparaitem}[$\circ$]\item \quotes{Yes,} \item \quotes{No,} \item \quotes{I prefer not to answer,} \item \quotes{Other (*required: please specify)} \end{inparaitem} \par  
    \vspace{4pt}

    \item \textbf{Q. 5} Where do you live?  \par
    \textbf{Answers:} \begin{inparaitem}[$\circ$]\item \quotes{Saudi Arabia,} \item \quotes{Other (*required: please specify)} \end{inparaitem} \par 
    \vspace{4pt}

    \item \textbf{Q. 6} In which region of Saudi Arabia do you live?  \par
    \textbf{Answers:} \begin{inparaitem}[$\circ$]\item \quotes{Western,} \item \quotes{Eastern,} \item \quotes{Central,} \item \quotes{Northern,} \item \quotes{Southern,} \item \quotes{Other (*required: please specify)} \end{inparaitem} \par 
    \vspace{4pt}

    \item \textbf{Q. 7} What is the highest academic degree you completed?  \par
    \textbf{Answers:} \begin{inparaitem}[$\circ$]\item \quotes{Doctorate,} \item \quotes{Masters,} \item \quotes{Bachelor,} \item \quotes{High school,} \item \quotes{Middle school,} \item \quotes{Elementary school,} \item \quotes{Other (*required: please specify)} \end{inparaitem} \par 
    \vspace{4pt}

    \item \textbf{Q. 8} \textbf{[If Q. 7 answer was \quotes{Doctorate}]} What is your major for the Doctorate degree? \par
    \textbf{Answers:} Open	\par 
    \vspace{4pt}

    \item \textbf{Q. 9} \textbf{[If Q. 7 answer was \quotes{Doctorate} or \quotes{Masters}]} What is your major for the Masters degree? \par
    \textbf{Answers:} Open	\par 
    \vspace{4pt}

    \item \textbf{Q. 10} \textbf{[If Q. 7 answer was \quotes{Doctorate} or \quotes{Masters} or \quotes{Bachelor}]} What is your major for the Bachelor degree? \par
    \textbf{Answers:} Open	\par 
    \vspace{4pt}

    \item \textbf{Q. 11} \textbf{[If Q. 7 answer was \quotes{Doctorate} or \quotes{Masters} or \quotes{Bachelor}]} What is your major for the Bachelor degree? \par
    \textbf{Answers:} Open	\par 
    \vspace{4pt}

    \item \textbf{Q. 12} What is your current employment status? \par 
    \textbf{Answers:} \begin{inparaitem}[$\circ$]\item \quotes{Student,} \item \quotes{Full-time employee,} \item \quotes{Part-time employee,} \item \quotes{Self-employed or business owner,} \item \quotes{Full-time house wife/husband,} \item \quotes{Unemployed, and looking for a job,} \item \quotes{Unemployed and, and not looking for a job,} \item \quotes{Unable to work,} \item \quotes{Retired,} \item \quotes{Other (*required: please specify)} \end{inparaitem}\par 
    \vspace{4pt}

    \item \textbf{Q. 13} \textbf{[If Q. 12 answer was \quotes{Student}]} If you are a student, what is the degree you are currently studying? \par 
    \textbf{Answers:} \begin{inparaitem}[$\circ$]\item \quotes{Doctorate,} \item \quotes{Masters,} \item \quotes{Bachelor,} \item \quotes{High school,} \item \quotes{Other (*required: please specify)} \end{inparaitem}\par 
    \vspace{4pt}

    \item \textbf{Q. 14} \textbf{[If Q. 12 answer was \quotes{Student} and Q. 13 answer was \quotes{Doctorate}]} What is the major you are currently studying in the Doctorate degree?
    \textbf{Answers:} Open	\par 
    \vspace{4pt}

    \item \textbf{Q. 15} \textbf{[If Q. 12 answer was \quotes{Student} and Q. 13 answer was \quotes{Masters}]} What is the major you are currently studying in the Masters degree?
    \textbf{Answers:} Open	\par 
    \vspace{4pt}

    \item \textbf{Q. 16} \textbf{[If Q. 12 answer was \quotes{Student} and Q. 13 answer was \quotes{Bachelor}]} What is the major you are currently studying in the Bachelor degree?
    \textbf{Answers:} Open	\par 
    \vspace{4pt}

    \item \textbf{Q. 17} Do you have a degree or work on Computer Science, Information Systems, Information Technology, or Computer Engineering? \par 
    \textbf{Answers:} \begin{inparaitem}[$\circ$]\item \quotes{Yes,} \item \quotes{No} \end{inparaitem} \par 
    \vspace{4pt}

    \item \textbf{Q. 18} \textbf{[If Q. 12 answer was \quotes{Full-time employee} or \quotes{Part-time employee} or \quotes{Self-employed or business owner}]} What is the sector you are currently working on? \par 
    \textbf{Answers:} \begin{inparaitem}[$\circ$]\item \quotes{Education (pre-university),} \item \quotes{University Education,} \item \quotes{Health,}  \item \quotes{Communication and Information Technology,} \item \quotes{Financial,} \item \quotes{Industrial,} \item \quotes{Agricultural,} \item \quotes{Sales and retail,} \item \quotes{Petrochemical,} \item \quotes{Other (*required: please specify)}  \end{inparaitem} \par 
    \vspace{4pt}
    
    \item \textbf{Q. 19} \textbf{[If Q. 12 answer was \quotes{Retired}]} What is the sector you worked on for your last job? \par 
    \textbf{Answers:} \begin{inparaitem}[$\circ$]\item \quotes{Education (pre-university),} \item \quotes{University Education,} \item \quotes{Health,}  \item \quotes{Communication and Information Technology,} \item \quotes{Financial,} \item \quotes{Industrial,} \item \quotes{Agricultural,} \item \quotes{Sales and retail,} \item \quotes{Petrochemical,} \item \quotes{Other (*required: please specify)}  \end{inparaitem} \par 
    \vspace{4pt} \par 

    \item \textbf{Q. 20} \textbf{[If Q. 12 answer was \quotes{Full-time employee} or \quotes{Part-time employee} or \quotes{Self-employed or business owner}]} What is your current job title? (e.g. Teacher, Assistant Professor, Doctor, Nurse, etc.)? \par
   \textbf{Answers:} Open	\par 
    \vspace{4pt}

    \item \textbf{Q. 21} \textbf{[If Q. 12 answer was \quotes{Retired}]} What is your job title in your last job? (e.g. Teacher, Assistant Professor, Doctor, Nurse, etc.)? \par
   \textbf{Answers:} Open	\par 
    \vspace{4pt}

    \item \textbf{Q. 22} What is your rate for your English language proficiency level?
    \par 
    \textbf{Answers:} \begin{inparaitem}[$\circ$]\item \quotes{Advanced (fluent in English),} \item \quotes{Above average (I rarely need to search for words),} \item \quotes{Average (Sometimes I need to search for some words),} \item \quotes{Below average (Mostly, I need to search for some words),} \item \quotes{Beginner (I know some common words),} \item \quotes{I do not know English at all} \end{inparaitem}

    \item \textbf{Q. 23} Approximately, when did you start using this email (that you used in the interview experiment)? \par 
     \textbf{Answers:} \begin{inparaitem}[$\circ$]\item \quotes{At least since a month,} \item \quotes{At least since 3 months,} \item \quotes{At least since 6 months,} \item \quotes{At least since a year,} \item \quotes{At least since 2 years,} \item \quotes{At least since 3 years,} \item \quotes{At least since 4 years,} \item \quotes{At least since 5 years,} \item \quotes{At least since more than 5 years,} \item \quotes{Other (*required: please specify)}\end{inparaitem}

    \item \textbf{Q. 24} What is the browser that you mostly use when you browse the Internet? \par 
     \textbf{Answers:} \begin{inparaitem}[$\circ$]\item \quotes{Google Chrome,} \item \quotes{Firefox,} \item \quotes{Brave,} \item \quotes{MS Edge,} \item \quotes{Safari,} \item \quotes{Opera,} \item \quotes{Other (*required: please specify)}\end{inparaitem}
     
\end{itemize}
