# Supplementary material for: Privacy Perceptions and Behaviors of Google Personal Account Holders in Saudi Arabia
Source: arXiv:2308.10148 source file (2024-08-07)
Supplement: Supplementary file 5 [file more_related.tex]

\section{More Background} \label{app:background}
%=========== BEGIN MORE OPTIONS FIG =====================
\begin{figure}[!th] %{r}{0.4\textwidth}
    %\vspace{-8mm}
	\begin{center}
	\includegraphics[width=0.4\textwidth]{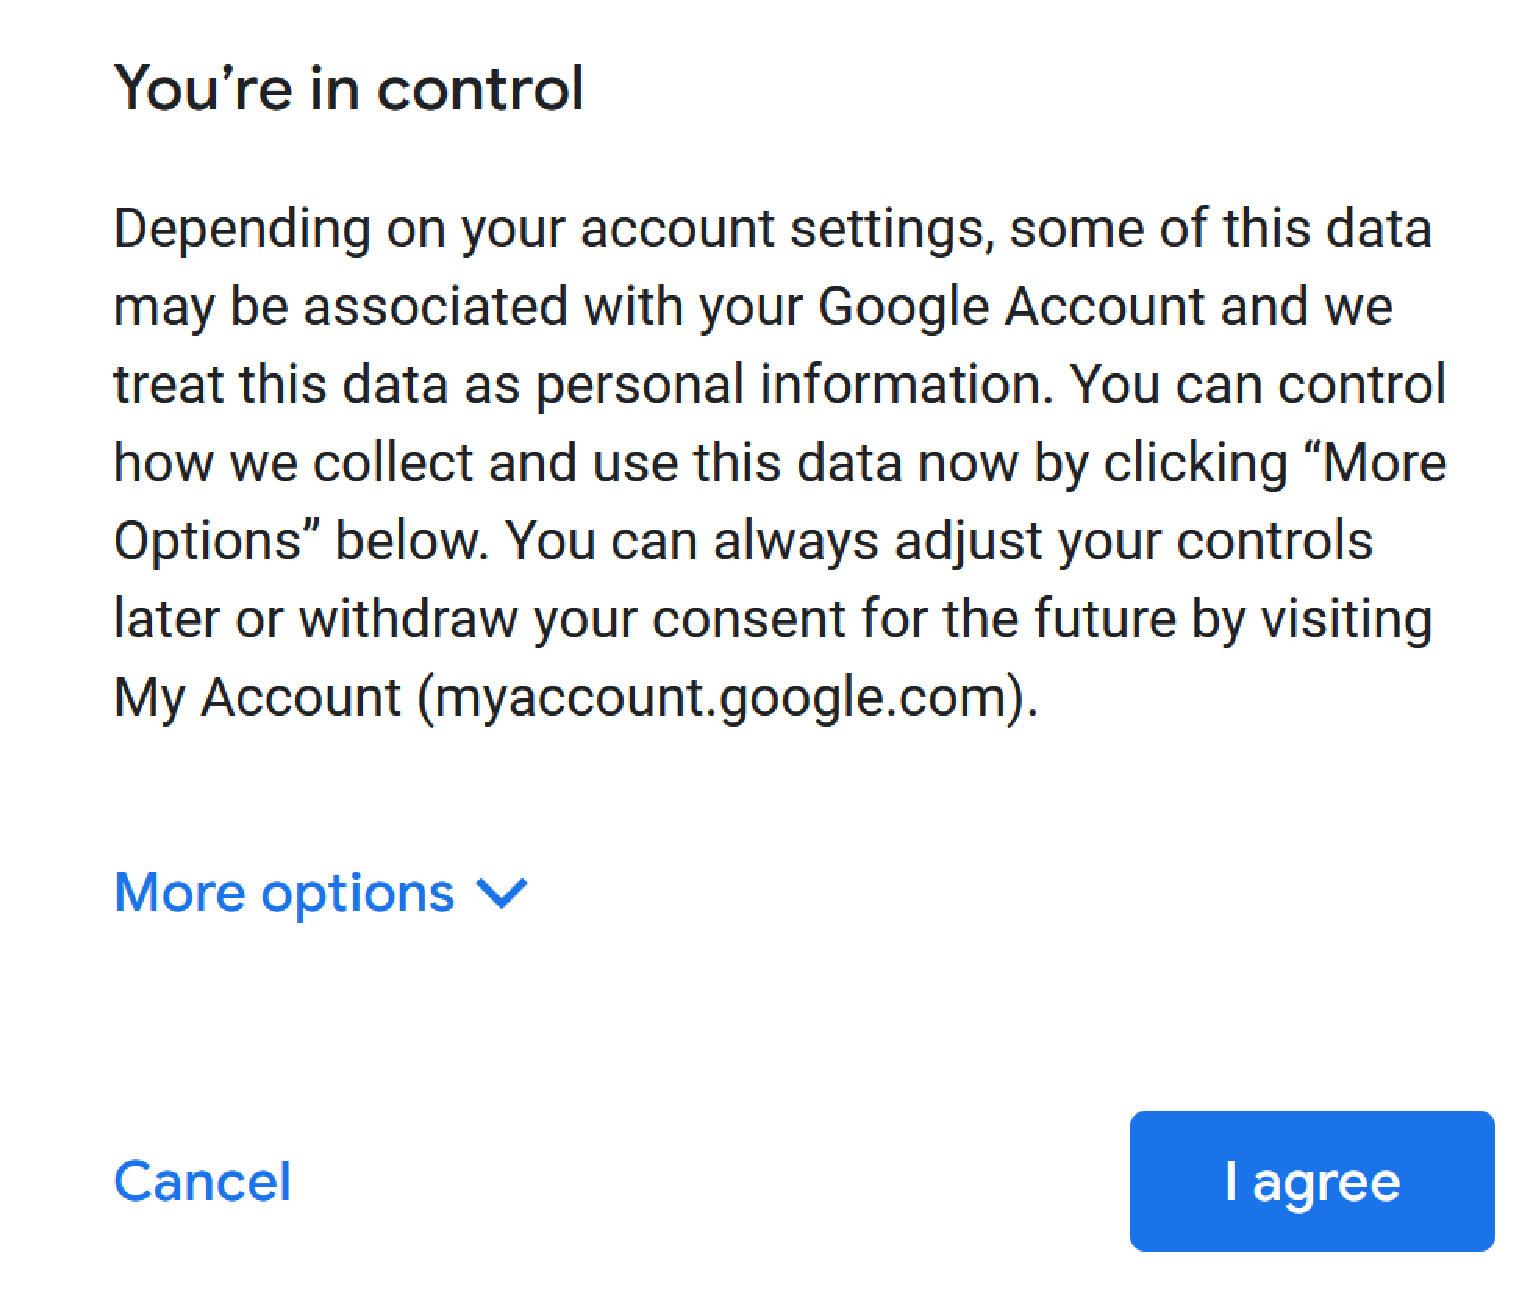}
    \end{center}
	\caption{Google's \quotes{Privacy and Terms} page which appears during the sign-up process. Only if the \quotes{More options} link is clicked, users can change the permissive default privacy settings.}
	\label{fig:options}
	\vspace{-8mm}
\end{figure}
%=========== END MORE OPTIONS FIG ===================== 
