# Supplementary material for: Privacy Perceptions and Behaviors of Google Personal Account Holders in Saudi Arabia
Source: arXiv:2308.10148 source file (2024-08-07)
Supplement: Supplementary file 7 [file questions_closing.tex]

\subsection{Closing Questions}
\begin{itemize}
\item \textbf{Q.} Do you have any degree or work on the cyber security area? \par
	\textbf{Answers:} \begin{inparaitem}[$\circ$] \item \quotes{Yes,} \item \quotes{No}  \end{inparaitem}
\vspace{4pt}
\item \textbf{Q.} Do you believe you learned something from the interview?\par 
	\textbf{Answers:} Open
\vspace{4pt}
\item \textbf{Q.} Are there any questions you expected us to ask you? \par 
    \textbf{Answers:} Open
\vspace{4pt}
\item \textbf{Q.} Are there any additional information related to the interview topic you would like to say? \par 
    \textbf{Answers:} Open
 \vspace{4pt}   
\item \textbf{Q.} Can you nominate other participants? \par
    \textbf{Answers:} Open
\end{itemize}
%-------------------------------------------------
